# Supplementary material for: Privacy in geo-social networks: proximity notification with untrusted service providers and curious buddies
Source: arXiv:1007.0408 source file (2010-11-06)
Supplement: Supplementary file 1 [file sec-appendix.tex]

\appendix

\section{Proof of formal results}

\subsection{Thoughts about the proofs}
In general, to prove the correctness of our protocols,
we need that for each user $u$ and each
set $M$ of generated messages
\[\forall l \in R \; pri(l) = post(l)\]
where $R$ is the uncertainty region
required by $u$ where $u$ is located.
Let rewrite $pri$ and $post$ with all the parameters
they need:
\[\forall l \in R \; pri(l, R) = post(l, R, M)\]

Now, let start assuming the privacy with respect to the SP.
In this case, $R = W$ ($W$ is the entire world).
By definition of $pri$ and $post$,
\[pri(l, W) = P[loc(u) = l | l \in W] = P[loc(u)]\]
and
\[post(l, W, M) = P[loc(u) = l | l \in W \land \Gamma_M] = P[loc(u) | \Gamma_M] \]

Hence, we need to show that for each possible set of requests $\bar{M}$:
\[P[loc(u) = l] = P[loc(u) | M = \bar{M}]\]

Now, given that $M = \{m_1, \ldots , m_n\}$,
and $\bar{M} = \{\bar{m_1}, \ldots , \bar{m_n}\}$
we need to show that:
\[P[loc(u) = l] = P[loc(u) =l | m_1 = \bar{m_1}, \land \ldots \land m_n = \bar{m_n}]\]

Here we have a first problem: can we find a sufficient condition
about the independence between the events $loc(u) = l$,
$m_1 = \bar{m_1}$, $\ldots$, $m_n = \bar{m_n}$
such that the equation above holds?

In other words, under which relationships between
events $A$, $B$, $C$, $D$, the following equation holds?
\[P[A | B \land C \land D] = P[A]\]

Once we have this result, we can show, for each of our protocols,
that they generate a set of messages with the required properties.
To do that, if necessary, we can examine the content of each request,
dividing it into \emph{IDdata}, \emph{TimeData} and \emph{MessageContent}.

\subsection{Proof for the \chns protocol with respect to the SP}
\begin{theorem}
Let $M$ be a set of messages exchanged during the execution of \chns.
Let $u$ be a user.
Given that $k_u$ is not known, for each location $l$,
\[pri(l, W) = post(l, W, M)\]
\end{theorem}

\begin{proof}
By definition of $pri$ and $post$,
\[pri(l, W) = P[loc(u) = l | l \in W] = P[loc(u)]\]
and
\[post(l, W, M) = P[loc(u) = l | l \in W \land \Gamma_M] = P[loc(u) | \Gamma_M] \]

Hence, we need to show that:
\[P[loc(u) = l] = P[loc(u)=l | \Gamma_M]\]

\textbf{This first part may be common for all the proofs wrt to the SP}

For a single request $m$
the equation 
\[P[loc(u) = l] = P[loc(u)=l | \Gamma_m]\]
holds because $\Gamma_m$ is independent from $loc(u)=l$.
\textbf{How to formalize it?}

\end{proof}

\subsection{Proof of Theorem~\ref{th:hnsSP}}

\begin{proof}

\end{proof}

\subsection{Proof of Theorem~\ref{th:hnsbuddies}}

\begin{proof}

\end{proof}
